# Supplementary material for: IW And-Type State in IM Eridani
Source: arXiv:1911.01587 ancillary file (2019-11-05)
Supplement: Supplementary file 1 [file si.pdf]

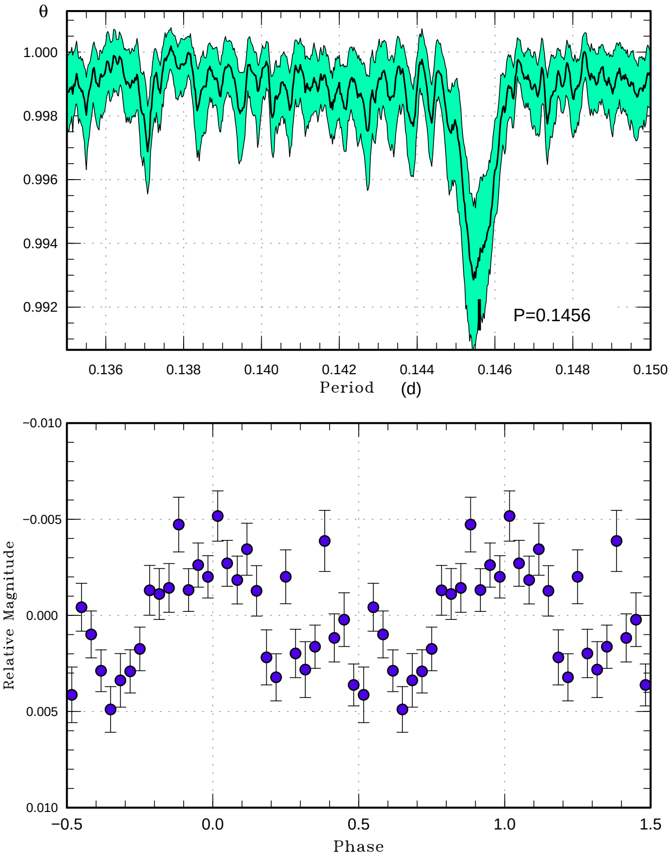


**E-figure 1.** PDM analysis of IM Eri before BJD 2458430 (oscillation phase before TO1).

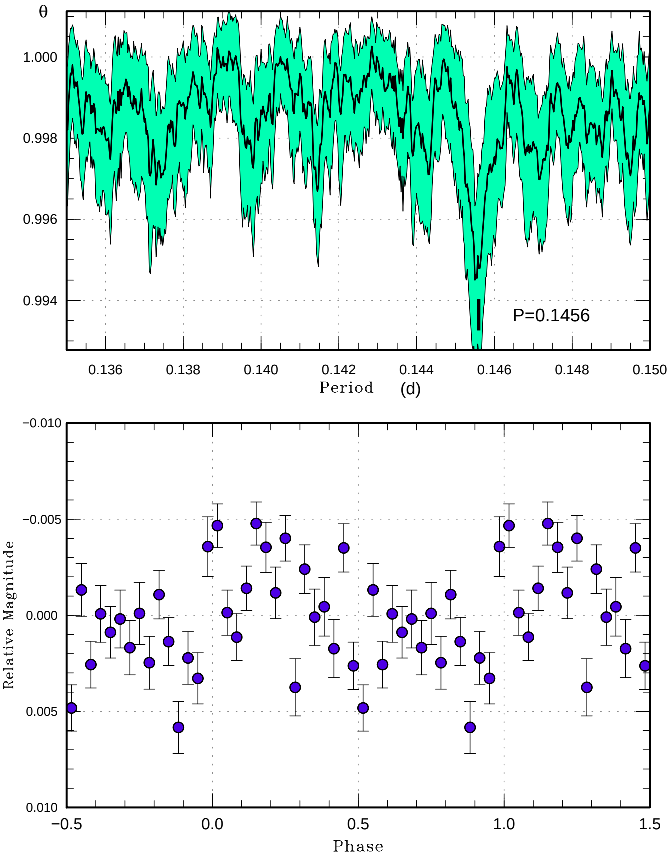


**E-figure 2.** PDM analysis of IM Eri between BJD 2458440 and 2458474 (oscillation phase between TO1 and TO2).

**E-table 1.** Log of Observations

| Start* | End* | Mean mag | error | $N^\dagger$ | Observer‡ | Filter |
|---|---|---|---|---|---|---|
| 58404.2375 | 58404.2403 | -0.157 | 0.002 | 5 | KU1 | C |
| 58404.5622 | 58404.7209 | 12.126 | 0.010 | 102 | Van | V |
| 58404.5687 | 58404.6163 | 0.535 | 0.002 | 228 | CRI | C |
| 58404.6337 | 58404.8638 | 12.252 | 0.005 | 96 | HaC | V |
| 58406.5693 | 58406.6844 | 12.069 | 0.003 | 138 | Van | CV |
| 58406.6568 | 58406.8627 | 11.885 | 0.006 | 85 | HaC | V |
| 58407.1294 | 58407.2294 | -0.397 | 0.002 | 245 | OKU | C |
| 58407.6539 | 58407.8620 | 11.687 | 0.002 | 86 | HaC | V |
| 58408.5914 | 58408.7394 | 11.896 | 0.006 | 89 | Van | CV |
| 58408.6513 | 58408.8612 | 11.846 | 0.004 | 87 | HaC | V |
| 58409.1749 | 58409.1777 | -0.162 | 0.002 | 5 | KU1 | C |
| 58409.2133 | 58409.3337 | -0.220 | 0.003 | 240 | OKU | C |
| 58409.6486 | 58409.8604 | 12.128 | 0.005 | 92 | HaC | V |
| 58410.1033 | 58410.2207 | 0.025 | 0.002 | 271 | OKU | C |
| 58410.1389 | 58410.1842 | -2.743 | 0.004 | 64 | KU2 | C |
| 58410.6459 | 58410.8599 | 12.095 | 0.004 | 93 | HaC | V |
| 58411.1057 | 58411.3061 | -0.222 | 0.002 | 490 | OKU | C |
| 58411.1304 | 58411.1786 | -2.945 | 0.004 | 67 | KU2 | C |
| 58411.5427 | 58411.7075 | 11.990 | 0.003 | 131 | Van | CV |
| 58411.6429 | 58411.8591 | 11.880 | 0.003 | 94 | HaC | V |
| 58412.0933 | 58412.1877 | -0.342 | 0.002 | 234 | OKU | C |
| 58412.1139 | 58412.3408 | 11.870 | 0.002 | 345 | Ioh | V |
| 58412.1181 | 58412.1888 | -3.120 | 0.004 | 99 | KU2 | C |
| 58412.6401 | 58412.8583 | 11.914 | 0.003 | 91 | HaC | V |
| 58413.0806 | 58413.2852 | -0.190 | 0.002 | 494 | OKU | C |
| 58413.1358 | 58413.2925 | 11.986 | 0.003 | 241 | Ioh | V |
| 58413.6345 | 58413.8599 | 12.118 | 0.004 | 94 | HaC | V |
| 58414.1082 | 58414.1836 | -0.037 | 0.003 | 166 | OKU | C |
| 58414.1183 | 58414.1820 | -2.807 | 0.007 | 91 | KU2 | C |
| 58414.6345 | 58414.8571 | 12.050 | 0.004 | 93 | HaC | V |
| 58415.5290 | 58415.6403 | 11.989 | 0.002 | 147 | Van | CV |
| 58415.6316 | 58415.8564 | 11.846 | 0.004 | 94 | HaC | V |
| 58416.0826 | 58416.1669 | -0.354 | 0.001 | 207 | OKU | C |
| 58416.5530 | 58416.6077 | 11.967 | 0.001 | 213 | Van | CV |
| 58416.6283 | 58416.8556 | 11.883 | 0.006 | 90 | HaC | V |
| 58417.0770 | 58417.1646 | -0.278 | 0.002 | 218 | OKU | C |
| 58417.6261 | 58417.8551 | 12.072 | 0.005 | 96 | HaC | V |
| 58418.6237 | 58418.8545 | 12.110 | 0.005 | 97 | HaC | V |
| 58419.0725 | 58419.2927 | -0.191 | 0.002 | 531 | OKU | C |
| 58419.1274 | 58419.3478 | 11.982 | 0.004 | 161 | Ioh | V |
| 58419.1572 | 58419.1600 | -2.972 | 0.012 | 5 | KU2 | C |
| 58419.5440 | 58419.5994 | 11.969 | 0.002 | 229 | Van | CV |
| 58419.6206 | 58419.8536 | 11.868 | 0.003 | 98 | HaC | V |
| 58420.0719 | 58420.2924 | -0.354 | 0.002 | 281 | OKU | C |
| 58420.1686 | 58420.1990 | -3.091 | 0.007 | 44 | KU2 | C |
| 58420.5668 | 58420.6456 | 11.892 | 0.002 | 264 | Van | CV |
| 58420.6141 | 58420.8533 | 11.810 | 0.003 | 100 | HaC | V |

*BJD

†Number of observations.

‡Observer's code and zero-point correction values used in analysis (observations with magnitude larger than 10 reported real magnitudes and others reported differential ones; correction values smaller than −3 and larger than 10 correspond to these two types of observations, respectively): CRI (Crimean Astrophys. Obs., 6.284), DKS (Dvorak, −5.301), HaC (Hambsch, −5.324), Ioh (Itoh, −5.346), KU1 (Kyoto U., 6.813), KU2 (Kyoto U., 9.604), MLF (Monard, 6.294), OKU (Osaka Kyoiku U., 6.845), Van (Vanmunster, −5.292 for V and −5.401 for CV.

**E-table 1.** Log of Observations (continued)

| Start* | End* | Mean mag | error | $N^{\dagger}$ | Observer‡ | Filter |
|---|---|---|---|---|---|---|
| 58421.0708 | 58421.1555 | -0.292 | 0.002 | 212 | OKU | C |
| 58421.6144 | 58421.8524 | 11.977 | 0.004 | 100 | HaC | V |
| 58421.7043 | 58421.8228 | 11.952 | 0.002 | 339 | DKS | V |
| 58422.0367 | 58422.1707 | 12.056 | 0.003 | 183 | Ioh | V |
| 58422.0771 | 58422.1923 | -0.122 | 0.002 | 233 | OKU | C |
| 58422.0986 | 58422.1382 | -2.871 | 0.007 | 32 | KU2 | C |
| 58422.6125 | 58422.8479 | 12.061 | 0.003 | 99 | HaC | V |
| 58423.0652 | 58423.1571 | -0.161 | 0.001 | 221 | OKU | C |
| 58423.6100 | 58423.8472 | 11.872 | 0.004 | 100 | HaC | V |
| 58424.0581 | 58424.1027 | -0.359 | 0.004 | 97 | OKU | C |
| 58424.2164 | 58424.3447 | 11.807 | 0.002 | 202 | Ioh | V |
| 58424.3848 | 58424.4336 | 0.193 | 0.001 | 129 | CRI | C |
| 58424.5633 | 58424.6225 | 11.907 | 0.006 | 167 | Van | CV |
| 58424.6074 | 58424.8468 | 11.778 | 0.002 | 101 | HaC | V |
| 58425.0547 | 58425.2442 | -0.385 | 0.004 | 74 | OKU | C |
| 58425.0863 | 58425.1681 | -3.217 | 0.004 | 94 | KU2 | C |
| 58425.1432 | 58425.3380 | 11.806 | 0.002 | 290 | Ioh | V |
| 58425.3832 | 58425.5751 | 0.209 | 0.001 | 491 | CRI | C |
| 58425.5362 | 58425.5999 | 11.874 | 0.003 | 216 | Van | CV |
| 58425.6047 | 58425.8468 | 11.849 | 0.003 | 102 | HaC | V |
| 58426.0549 | 58426.1032 | -0.244 | 0.002 | 158 | OKU | C |
| 58426.0862 | 58426.1501 | 11.928 | 0.004 | 60 | Ioh | V |
| 58426.8156 | 58426.8469 | 12.069 | 0.008 | 16 | HaC | V |
| 58427.0558 | 58427.0880 | -0.061 | 0.003 | 80 | OKU | C |
| 58427.3831 | 58427.6159 | 0.495 | 0.003 | 399 | CRI | C |
| 58427.5992 | 58427.8467 | 12.029 | 0.003 | 105 | HaC | V |
| 58428.4985 | 58428.5539 | 11.917 | 0.003 | 113 | Van | CV |
| 58428.5964 | 58428.8458 | 11.805 | 0.003 | 73 | HaC | V |
| 58429.0393 | 58429.1594 | -0.394 | 0.001 | 232 | OKU | C |
| 58429.4261 | 58429.4657 | 0.133 | 0.001 | 105 | CRI | C |
| 58429.5936 | 58429.8446 | 11.728 | 0.005 | 37 | HaC | V |
| 58430.0458 | 58430.1684 | -0.436 | 0.002 | 161 | OKU | C |
| 58430.4182 | 58430.5943 | 0.121 | 0.001 | 506 | MLF | C |
| 58430.5908 | 58430.8444 | 11.729 | 0.003 | 91 | HaC | V |
| 58430.5945 | 58430.6102 | 11.879 | 0.003 | 67 | Van | CV |
| 58431.7069 | 58431.8438 | 11.650 | 0.004 | 49 | HaC | V |
| 58432.4145 | 58432.5381 | -0.176 | 0.004 | 313 | CRI | C |
| 58432.7358 | 58432.8414 | 11.228 | 0.007 | 35 | HaC | V |
| 58433.0427 | 58433.1427 | -0.910 | 0.003 | 300 | OKU | C |
| 58433.3674 | 58433.5898 | -0.394 | 0.002 | 536 | CRI | C |
| 58433.7597 | 58433.8469 | 11.207 | 0.003 | 29 | HaC | V |
| 58434.0425 | 58434.0471 | -0.911 | 0.004 | 17 | OKU | C |
| 58434.7570 | 58434.8411 | 11.244 | 0.007 | 22 | HaC | V |
| 58435.7541 | 58435.8478 | 11.295 | 0.004 | 31 | HaC | V |
| 58436.0768 | 58436.2312 | -0.865 | 0.001 | 515 | OKU | C |
| 58436.7513 | 58436.8483 | 11.372 | 0.003 | 32 | HaC | V |
| 58437.0341 | 58437.1295 | 11.442 | 0.002 | 123 | Ioh | V |
| 58437.1097 | 58437.2703 | -0.719 | 0.001 | 477 | OKU | C |
| 58437.3324 | 58437.6011 | -0.047 | 0.001 | 770 | MLF | C |
| 58437.4038 | 58437.4374 | -0.059 | 0.005 | 80 | CRI | C |
| 58437.9963 | 58438.0779 | 11.755 | 0.003 | 99 | Ioh | V |
| 58438.0177 | 58438.2828 | -0.397 | 0.001 | 846 | OKU | C |
| 58438.7458 | 58438.8487 | 12.075 | 0.005 | 34 | HaC | V |
| 58439.7429 | 58439.8472 | 12.429 | 0.006 | 48 | HaC | V |
| 58440.0205 | 58440.2559 | 0.160 | 0.002 | 571 | OKU | C |
| 58440.7401 | 58440.8483 | 12.019 | 0.007 | 50 | HaC | V |

**E-table 1.** Log of Observations (continued)

| Start* | End* | Mean mag | error | $N^{\dagger}$ | Observer‡ | Filter |
|---|---|---|---|---|---|---|
| 58441.7374 | 58441.8469 | 11.741 | 0.003 | 51 | HaC | V |
| 58442.0423 | 58442.1334 | -0.435 | 0.002 | 51 | OKU | C |
| 58442.7346 | 58442.8465 | 11.865 | 0.004 | 52 | HaC | V |
| 58443.0018 | 58443.2665 | -0.232 | 0.001 | 898 | OKU | C |
| 58443.7322 | 58443.8461 | 12.168 | 0.006 | 53 | HaC | V |
| 58443.9994 | 58444.0091 | 0.126 | 0.006 | 23 | OKU | C |
| 58444.7294 | 58444.8471 | 12.396 | 0.005 | 55 | HaC | V |
| 58445.0496 | 58445.2746 | 0.010 | 0.002 | 632 | OKU | C |
| 58445.0587 | 58445.2814 | 12.216 | 0.005 | 203 | Ioh | V |
| 58445.7268 | 58445.8420 | 11.915 | 0.011 | 37 | HaC | V |
| 58446.0130 | 58446.0985 | -0.352 | 0.002 | 268 | OKU | C |
| 58446.7239 | 58446.8418 | 11.716 | 0.004 | 38 | HaC | V |
| 58446.9966 | 58447.2305 | -0.444 | 0.001 | 777 | OKU | C |
| 58447.7212 | 58447.8419 | 11.863 | 0.004 | 39 | HaC | V |
| 58448.1087 | 58448.2643 | 11.976 | 0.002 | 200 | Ioh | V |
| 58448.1135 | 58448.2276 | -0.219 | 0.001 | 393 | OKU | C |
| 58448.7183 | 58448.8421 | 12.133 | 0.006 | 40 | HaC | V |
| 58449.0615 | 58449.0921 | 12.244 | 0.007 | 36 | Ioh | V |
| 58449.7155 | 58449.8391 | 12.210 | 0.008 | 58 | HaC | V |
| 58450.0142 | 58450.0892 | 12.139 | 0.003 | 104 | Ioh | V |
| 58450.2305 | 58450.2331 | -0.086 | 0.006 | 10 | OKU | C |
| 58450.7129 | 58450.8367 | 11.873 | 0.004 | 40 | HaC | V |
| 58451.1742 | 58451.1774 | -0.374 | 0.006 | 9 | OKU | C |
| 58451.7101 | 58451.8367 | 11.744 | 0.004 | 41 | HaC | V |
| 58451.9750 | 58452.0843 | 11.762 | 0.003 | 151 | Ioh | V |
| 58451.9941 | 58452.0540 | -0.409 | 0.002 | 150 | OKU | C |
| 58452.7081 | 58452.8377 | 11.851 | 0.005 | 42 | HaC | V |
| 58453.0075 | 58453.1276 | -0.270 | 0.001 | 300 | OKU | C |
| 58453.1546 | 58453.2577 | 11.929 | 0.002 | 138 | Ioh | V |
| 58453.7054 | 58453.8381 | 12.069 | 0.006 | 43 | HaC | V |
| 58454.2071 | 58454.2107 | -0.023 | 0.004 | 10 | OKU | C |
| 58454.7023 | 58454.8376 | 12.126 | 0.006 | 44 | HaC | V |
| 58455.6995 | 58455.8377 | 11.884 | 0.004 | 45 | HaC | V |
| 58456.6967 | 58456.8377 | 11.757 | 0.004 | 46 | HaC | V |
| 58457.6940 | 58457.8379 | 11.794 | 0.004 | 47 | HaC | V |
| 58457.9387 | 58458.0728 | 11.848 | 0.003 | 110 | Ioh | V |
| 58458.0087 | 58458.1111 | -0.340 | 0.001 | 358 | OKU | C |
| 58458.8024 | 58458.8367 | 11.951 | 0.009 | 13 | HaC | V |
| 58459.6892 | 58459.8387 | 11.969 | 0.006 | 49 | HaC | V |
| 58460.6879 | 58460.8373 | 11.856 | 0.004 | 49 | HaC | V |
| 58461.0892 | 58461.1597 | 11.865 | 0.004 | 76 | Ioh | V |
| 58461.6851 | 58461.8373 | 11.809 | 0.005 | 50 | HaC | V |
| 58462.0629 | 58462.0712 | -0.358 | 0.003 | 30 | OKU | C |
| 58462.6823 | 58462.8375 | 11.812 | 0.003 | 51 | HaC | V |
| 58463.0956 | 58463.0982 | -0.375 | 0.005 | 10 | OKU | C |
| 58463.6795 | 58463.8376 | 11.829 | 0.004 | 52 | HaC | V |
| 58464.6768 | 58464.8377 | 11.891 | 0.005 | 53 | HaC | V |
| 58465.0791 | 58465.0806 | -0.306 | 0.004 | 10 | OKU | C |
| 58465.6774 | 58465.8349 | 11.897 | 0.004 | 52 | HaC | V |
| 58466.1665 | 58466.1681 | -0.291 | 0.005 | 10 | OKU | C |
| 58466.6685 | 58466.8386 | 11.818 | 0.005 | 56 | HaC | V |
| 58467.0814 | 58467.0829 | -0.349 | 0.006 | 6 | OKU | C |
| 58467.6657 | 58467.8384 | 11.791 | 0.003 | 57 | HaC | V |
| 58468.1021 | 58468.1036 | -0.425 | 0.004 | 10 | OKU | C |
| 58469.3226 | 58469.4582 | 11.971 | 0.002 | 483 | Van | CV |
| 58469.6602 | 58469.8387 | 11.903 | 0.004 | 59 | HaC | V |

**E-table 1.** Log of Observations (continued)

| Start* | End* | Mean mag | error | $N^\dagger$ | Observer‡ | Filter |
|---|---|---|---|---|---|---|
| 58470.1367 | 58470.1387 | -0.193 | 0.018 | 8 | OKU | C |
| 58470.6606 | 58470.8360 | 11.891 | 0.005 | 51 | HaC | V |
| 58471.0725 | 58471.0750 | -0.271 | 0.003 | 10 | OKU | C |
| 58471.6546 | 58471.8364 | 11.762 | 0.004 | 60 | HaC | V |
| 58472.5901 | 58472.8374 | 11.693 | 0.003 | 81 | HaC | V |
| 58473.5030 | 58473.5414 | 11.764 | 0.002 | 140 | Van | CV |
| 58473.5875 | 58473.8357 | 11.624 | 0.004 | 81 | HaC | V |
| 58474.5856 | 58474.8376 | 11.184 | 0.004 | 82 | HaC | V |
| 58475.0795 | 58475.0862 | -0.994 | 0.004 | 18 | OKU | C |
| 58475.4633 | 58475.5216 | 11.291 | 0.001 | 194 | Van | CV |
| 58475.5829 | 58475.8379 | 11.177 | 0.002 | 105 | HaC | V |
| 58476.5800 | 58476.8363 | 11.197 | 0.002 | 83 | HaC | V |
| 58477.1009 | 58477.1024 | -0.924 | 0.002 | 10 | OKU | C |
| 58477.5772 | 58477.8374 | 11.290 | 0.003 | 84 | HaC | V |
| 58478.0501 | 58478.0524 | -0.806 | 0.005 | 8 | OKU | C |
| 58478.5745 | 58478.8377 | 11.450 | 0.005 | 79 | HaC | V |
| 58479.5724 | 58479.8389 | 11.763 | 0.005 | 80 | HaC | V |
| 58480.0264 | 58480.0289 | -0.333 | 0.005 | 10 | OKU | C |
| 58480.5713 | 58480.8192 | 12.165 | 0.008 | 74 | HaC | V |
| 58481.5685 | 58481.8087 | 12.300 | 0.010 | 60 | HaC | V |
| 58483.3470 | 58483.4894 | 11.916 | 0.002 | 396 | Van | CV |
| 58483.5631 | 58483.8093 | 11.810 | 0.004 | 57 | HaC | V |
| 58484.3326 | 58484.4675 | 11.945 | 0.003 | 222 | Van | CV |
| 58486.3447 | 58486.4888 | 12.134 | 0.002 | 518 | Van | CV |
| 58488.5535 | 58488.7606 | 11.852 | 0.003 | 68 | HaC | V |
| 58489.5522 | 58489.7574 | 11.935 | 0.003 | 66 | HaC | V |
| 58490.0449 | 58490.0475 | -0.220 | 0.007 | 10 | OKU | C |
| 58490.3355 | 58490.4894 | 12.079 | 0.002 | 630 | Van | CV |
| 58490.5522 | 58490.7402 | 11.966 | 0.004 | 61 | HaC | V |
| 58491.5525 | 58491.7357 | 11.911 | 0.005 | 61 | HaC | V |
| 58492.0363 | 58492.0373 | -0.240 | 0.002 | 7 | OKU | C |
| 58492.3988 | 58492.4853 | 11.944 | 0.004 | 52 | Van | CV |
| 58492.6308 | 58492.7191 | 11.843 | 0.007 | 24 | HaC | V |
| 58493.0822 | 58493.0829 | -0.313 | 0.002 | 5 | OKU | C |
| 58493.3385 | 58493.4897 | 11.935 | 0.004 | 97 | Van | CV |
| 58493.5605 | 58493.7324 | 11.867 | 0.004 | 41 | HaC | V |
| 58494.5553 | 58494.7295 | 11.906 | 0.006 | 45 | HaC | V |
| 58495.6097 | 58495.7260 | 11.887 | 0.008 | 23 | HaC | V |
| 58496.0892 | 58496.0908 | -0.305 | 0.004 | 9 | OKU | C |
| 58496.4044 | 58496.4794 | 11.956 | 0.002 | 163 | Van | CV |
| 58496.5527 | 58496.7224 | 11.856 | 0.005 | 44 | HaC | V |
| 58497.0310 | 58497.0325 | -0.324 | 0.002 | 10 | OKU | C |
| 58497.3529 | 58497.4740 | 11.958 | 0.002 | 224 | Van | CV |
| 58497.5533 | 58497.7202 | 11.887 | 0.005 | 45 | HaC | V |
| 58498.0655 | 58498.0670 | -0.279 | 0.003 | 10 | OKU | C |
| 58498.3603 | 58498.4677 | 11.971 | 0.005 | 83 | Van | CV |
| 58498.5533 | 58498.7168 | 11.875 | 0.006 | 52 | HaC | V |
| 58499.5530 | 58499.7144 | 11.853 | 0.008 | 52 | HaC | V |
| 58500.0744 | 58500.0753 | -0.260 | 0.005 | 5 | OKU | C |
| 58502.0648 | 58502.0663 | -0.292 | 0.005 | 10 | OKU | C |
| 58503.0293 | 58503.0307 | -0.355 | 0.003 | 9 | OKU | C |
| 58503.5533 | 58503.7039 | 11.804 | 0.005 | 55 | HaC | V |
| 58504.5507 | 58504.7023 | 11.806 | 0.004 | 71 | HaC | V |
| 58505.0586 | 58505.0600 | -0.365 | 0.006 | 9 | OKU | C |
| 58505.3207 | 58505.4502 | 11.919 | 0.004 | 74 | Van | CV |
| 58505.5511 | 58505.6988 | 11.828 | 0.009 | 27 | HaC | V |

**E-table 1.** Log of Observations (continued)

| Start* | End* | Mean mag | error | $N^{\dagger}$ | Observer‡ | Filter |
|---|---|---|---|---|---|---|
| 58506.0652 | 58506.0667 | -0.284 | 0.003 | 10 | OKU | C |
| 58506.5503 | 58506.6961 | 11.804 | 0.005 | 56 | HaC | V |
| 58507.0694 | 58507.0707 | -0.242 | 0.006 | 8 | OKU | C |
| 58507.5501 | 58507.6705 | 11.799 | 0.006 | 45 | HaC | V |
| 58508.0725 | 58508.0738 | -0.353 | 0.005 | 9 | OKU | C |
| 58508.3304 | 58508.4476 | 11.886 | 0.001 | 489 | Van | CV |
| 58509.3477 | 58509.4409 | 11.898 | 0.004 | 57 | Van | CV |
| 58510.3326 | 58510.4397 | 11.882 | 0.003 | 61 | Van | CV |
| 58511.3508 | 58511.4373 | 11.898 | 0.002 | 367 | Van | CV |
| 58512.0124 | 58512.0132 | -0.394 | 0.007 | 5 | OKU | C |
| 58516.0253 | 58516.0268 | -0.629 | 0.002 | 10 | OKU | C |
| 58517.3271 | 58517.3342 | 11.266 | 0.012 | 5 | Van | CV |
| 58518.9770 | 58518.9785 | -0.861 | 0.003 | 10 | OKU | C |
| 58519.3204 | 58519.4269 | 11.388 | 0.002 | 206 | Van | CV |
| 58519.9824 | 58519.9839 | -0.844 | 0.004 | 10 | OKU | C |
| 58520.3187 | 58520.4168 | 11.491 | 0.002 | 103 | Van | CV |
| 58521.3208 | 58521.4270 | 11.732 | 0.003 | 61 | Van | CV |
| 58522.3186 | 58522.4153 | 12.011 | 0.004 | 69 | Van | CV |
| 58523.9284 | 58523.9310 | 0.028 | 0.009 | 8 | OKU | C |
| 58524.9416 | 58524.9439 | -0.240 | 0.003 | 9 | OKU | C |
| 58527.9365 | 58527.9378 | -0.197 | 0.005 | 10 | OKU | C |
| 58528.3171 | 58528.3402 | 12.078 | 0.002 | 98 | Van | CV |
| 58528.5295 | 58528.6359 | 11.961 | 0.005 | 39 | HaC | V |
| 58529.3254 | 58529.3888 | 11.971 | 0.002 | 264 | Van | CV |
| 58529.5393 | 58529.6336 | 11.872 | 0.004 | 46 | HaC | V |
| 58530.3064 | 58530.3886 | 11.963 | 0.002 | 339 | Van | CV |
| 58530.5383 | 58530.6300 | 11.859 | 0.005 | 44 | HaC | V |
| 58531.3259 | 58531.3852 | 12.016 | 0.002 | 247 | Van | CV |
| 58531.5386 | 58531.6275 | 11.899 | 0.007 | 34 | HaC | V |
| 58531.8969 | 58531.8977 | -0.279 | 0.003 | 6 | OKU | C |
| 58532.5380 | 58532.6241 | 11.881 | 0.007 | 33 | HaC | V |
| 58533.3174 | 58533.3781 | 11.986 | 0.003 | 188 | Van | CV |
| 58533.5376 | 58533.6211 | 11.894 | 0.006 | 32 | HaC | V |
| 58534.5367 | 58534.6195 | 11.896 | 0.008 | 32 | HaC | V |
| 58535.3178 | 58535.3782 | 11.969 | 0.002 | 197 | Van | CV |
| 58535.5366 | 58535.6173 | 11.849 | 0.005 | 39 | HaC | V |
| 58536.5395 | 58536.6152 | 11.848 | 0.005 | 25 | HaC | V |
| 58537.3189 | 58537.3750 | 11.973 | 0.003 | 192 | Van | CV |
| 58537.5393 | 58537.6115 | 11.824 | 0.006 | 33 | HaC | V |
| 58537.9430 | 58537.9444 | -0.280 | 0.006 | 10 | OKU | C |
| 58538.2980 | 58538.3683 | 11.935 | 0.005 | 64 | Van | CV |
| 58538.5388 | 58538.6082 | 11.805 | 0.004 | 32 | HaC | V |
| 58538.8958 | 58538.8970 | -0.346 | 0.005 | 9 | OKU | C |
| 58539.2984 | 58539.3645 | 11.917 | 0.001 | 272 | Van | CV |
| 58539.5381 | 58539.6050 | 11.812 | 0.007 | 31 | HaC | V |
| 58539.9036 | 58539.9061 | -0.416 | 0.004 | 10 | OKU | C |
| 58540.3001 | 58540.3643 | 11.899 | 0.002 | 260 | Van | CV |
| 58540.5157 | 58540.6007 | 11.799 | 0.010 | 20 | HaC | V |
| 58540.9002 | 58540.9016 | -0.374 | 0.003 | 10 | OKU | C |
| 58541.3150 | 58541.3608 | 11.874 | 0.003 | 195 | Van | CV |
| 58542.5095 | 58542.5696 | 11.820 | 0.010 | 13 | HaC | V |
| 58543.5085 | 58543.5926 | 11.807 | 0.008 | 26 | HaC | V |
| 58543.9202 | 58543.9216 | -0.278 | 0.008 | 10 | OKU | C |
| 58544.3014 | 58544.3608 | 11.936 | 0.002 | 247 | Van | CV |
| 58544.5038 | 58544.5915 | 11.792 | 0.010 | 19 | HaC | V |
| 58545.3026 | 58545.3506 | 11.905 | 0.002 | 167 | Van | CV |
| 58545.5030 | 58545.5870 | 11.801 | 0.006 | 26 | HaC | V |

**E-table 1.** Log of Observations (continued)

| Start* | End* | Mean mag | error | $N^{\dagger}$ | Observer‡ | Filter |
|---|---|---|---|---|---|---|
| 58546.3091 | 58546.3472 | 11.902 | 0.006 | 30 | Van | CV |
| 58546.5024 | 58546.5864 | 11.772 | 0.006 | 26 | HaC | V |
| 58547.5016 | 58547.5823 | 11.813 | 0.007 | 25 | HaC | V |
| 58547.9024 | 58547.9046 | -0.384 | 0.008 | 7 | OKU | C |
| 58548.5012 | 58548.5819 | 11.780 | 0.005 | 25 | HaC | V |
| 58549.5000 | 58549.5773 | 11.755 | 0.007 | 24 | HaC | V |
| 58550.4994 | 58550.5767 | 11.758 | 0.006 | 24 | HaC | V |
| 58550.9101 | 58550.9114 | -0.360 | 0.003 | 10 | OKU | C |
| 58551.3069 | 58551.3367 | 11.900 | 0.002 | 113 | Van | CV |
| 58551.4989 | 58551.5729 | 11.739 | 0.005 | 23 | HaC | V |
| 58551.9105 | 58551.9117 | -0.377 | 0.005 | 7 | OKU | C |
| 58552.3061 | 58552.3331 | 11.852 | 0.003 | 97 | Van | CV |
| 58552.4981 | 58552.5686 | 11.732 | 0.006 | 22 | HaC | V |
| 58553.3061 | 58553.3298 | 11.841 | 0.002 | 99 | Van | CV |
| 58553.4977 | 58553.5682 | 11.736 | 0.006 | 22 | HaC | V |
| 58554.3129 | 58554.3263 | 11.803 | 0.002 | 55 | Van | CV |
| 58554.4967 | 58554.5640 | 11.707 | 0.005 | 21 | HaC | V |
| 58554.9178 | 58554.9189 | -0.405 | 0.015 | 5 | OKU | C |
| 58555.3060 | 58555.3227 | 11.755 | 0.003 | 75 | Van | CV |
| 58555.4962 | 58555.5600 | 11.680 | 0.007 | 20 | HaC | V |
| 58555.9109 | 58555.9121 | -0.516 | 0.004 | 9 | OKU | C |
| 58556.3074 | 58556.3227 | 11.809 | 0.004 | 68 | Van | CV |
| 58556.4952 | 58556.5589 | 11.734 | 0.006 | 20 | HaC | V |
| 58557.3096 | 58557.3192 | 11.884 | 0.005 | 38 | Van | CV |
| 58557.4946 | 58557.5552 | 11.703 | 0.006 | 19 | HaC | V |
| 58558.3094 | 58558.3194 | 11.875 | 0.003 | 43 | Van | CV |
| 58558.4939 | 58558.5543 | 11.706 | 0.006 | 19 | HaC | V |
| 58559.3099 | 58559.3192 | 11.872 | 0.003 | 36 | Van | CV |
| 58559.4932 | 58559.5502 | 11.728 | 0.005 | 18 | HaC | V |
| 58559.9135 | 58559.9149 | -0.378 | 0.004 | 10 | OKU | C |
| 58560.3109 | 58560.3194 | 11.897 | 0.004 | 37 | Van | CV |
| 58560.4920 | 58560.5472 | 11.785 | 0.005 | 21 | HaC | V |
| 58561.3130 | 58561.3189 | 11.875 | 0.004 | 25 | Van | CV |
| 58561.4909 | 58561.5464 | 11.767 | 0.005 | 21 | HaC | V |
| 58562.3137 | 58562.3183 | 11.897 | 0.012 | 10 | Van | CV |
| 58562.4904 | 58562.5412 | 11.788 | 0.006 | 22 | HaC | V |
| 58563.3400 | 58563.3435 | 11.934 | 0.015 | 10 | Van | CV |
| 58563.4923 | 58563.5408 | 11.775 | 0.009 | 21 | HaC | V |
| 58564.3305 | 58564.3349 | 11.895 | 0.008 | 16 | Van | CV |
| 58564.4893 | 58564.5379 | 11.787 | 0.005 | 21 | HaC | V |
| 58565.4886 | 58565.5347 | 11.805 | 0.007 | 20 | HaC | V |
| 58566.3308 | 58566.3368 | 11.976 | 0.013 | 19 | Van | CV |
| 58566.4882 | 58566.5309 | 11.774 | 0.003 | 15 | HaC | V |
| 58566.9185 | 58566.9199 | -0.350 | 0.002 | 10 | OKU | C |
| 58567.3318 | 58567.3366 | 12.087 | 0.018 | 8 | Van | CV |
| 58567.4872 | 58567.5269 | 11.781 | 0.005 | 14 | HaC | V |
| 58568.3209 | 58568.3367 | 11.961 | 0.006 | 53 | Van | CV |
| 58568.4865 | 58568.5263 | 11.758 | 0.007 | 14 | HaC | V |
| 58568.9239 | 58568.9245 | -0.231 | 0.026 | 4 | OKU | C |
| 58569.3241 | 58569.3331 | 11.865 | 0.012 | 20 | Van | CV |
| 58569.4854 | 58569.5246 | 11.743 | 0.007 | 14 | HaC | V |
| 58570.4836 | 58570.5191 | 11.754 | 0.008 | 11 | HaC | V |
| 58571.4849 | 58571.5169 | 11.703 | 0.009 | 10 | HaC | V |
| 58572.4839 | 58572.5159 | 11.721 | 0.009 | 10 | HaC | V |
| 58573.4829 | 58573.5112 | 11.736 | 0.007 | 9 | HaC | V |
| 58574.4863 | 58574.5005 | 11.765 | 0.010 | 4 | HaC | V |
| 58575.4817 | 58575.5065 | 11.774 | 0.008 | 4 | HaC | V |

**E-table 1.** Log of Observations (continued)

| Start* | End* | Mean mag | error | $N^\dagger$ | Observer‡ | Filter |
|---|---|---|---|---|---|---|
| 58576.3203 | 58576.3297 | 12.018 | 0.007 | 39 | Van | CV |
| 58576.4809 | 58576.5023 | 11.813 | 0.009 | 7 | HaC | V |
| 58578.4799 | 58578.5149 | 11.817 | 0.014 | 11 | HaC | V |
| 58579.4788 | 58579.5245 | 11.807 | 0.009 | 14 | HaC | V |
| 58580.4784 | 58580.5240 | 11.805 | 0.007 | 14 | HaC | V |
| 58582.4786 | 58582.5163 | 11.818 | 0.009 | 10 | HaC | V |
| 58583.4783 | 58583.5159 | 11.792 | 0.006 | 10 | HaC | V |
| 58584.4775 | 58584.5109 | 11.815 | 0.007 | 9 | HaC | V |
| 58585.4771 | 58585.5105 | 11.771 | 0.011 | 9 | HaC | V |
| 58586.4764 | 58586.5056 | 11.724 | 0.006 | 8 | HaC | V |
| 58587.4758 | 58587.5049 | 11.743 | 0.011 | 8 | HaC | V |
| 58588.4749 | 58588.4999 | 11.749 | 0.015 | 7 | HaC | V |
| 58590.4742 | 58590.4952 | 11.751 | 0.031 | 5 | HaC | V |
| 58591.4735 | 58591.4946 | 11.739 | 0.014 | 7 | HaC | V |
| 58592.4729 | 58592.4905 | 11.707 | 0.013 | 6 | HaC | V |
| 58593.4728 | 58593.4868 | 11.691 | 0.015 | 5 | HaC | V |
| 58594.4719 | 58594.4860 | 11.730 | 0.025 | 5 | HaC | V |
| 58595.4713 | 58595.4819 | 11.731 | 0.012 | 4 | HaC | V |
| 58596.4705 | 58596.4811 | 11.735 | 0.006 | 4 | HaC | V |
| 58598.4695 | 58598.4731 | 11.653 | 0.035 | 2 | HaC | V |
